# Supplementary material for: Visually Grounded Speech Models for Low-resource Languages and Cognitive Modelling
Source: arXiv:2409.02865 source file (2024-09-03)
Supplement: Supplementary file 2 [file appendices.tex]

\input{appendices/an_appendix}
